# Supplementary material for: Selectively Informative Description can Reduce Undesired Embedding Entanglements in Text-to-Image Personalization
Source: arXiv:2403.15330 source file (2024-03-22)
Supplement: Supplementary file 2 [file 937_1.Multi_vs_DB_diverse_but.tex]

\begin{figure*}[t]
    \centering
    \includegraphics[width=0.9\textwidth]{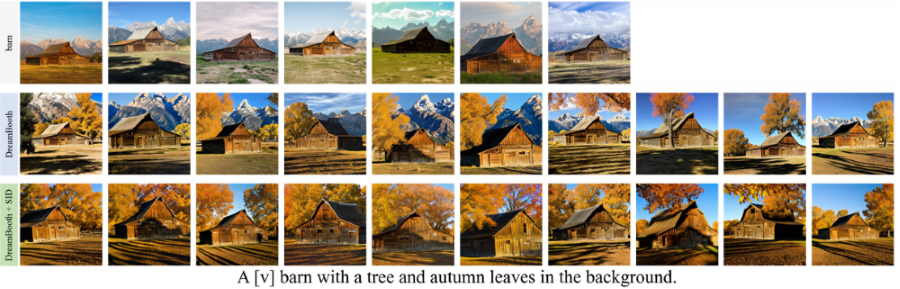}
    \vspace{0.2cm}

    \includegraphics[width=0.9\textwidth]{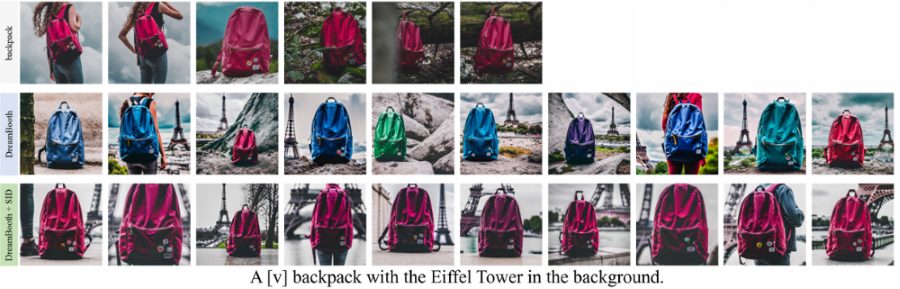}
    \vspace{0.2cm}

    \includegraphics[width=0.9\textwidth]{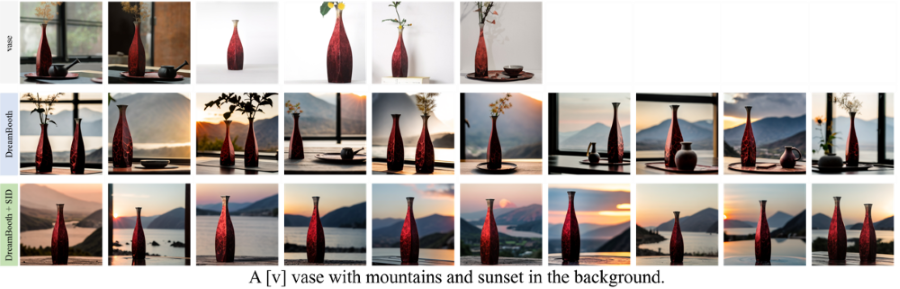}
    \vspace{0.2cm}

    \includegraphics[width=0.9\textwidth]{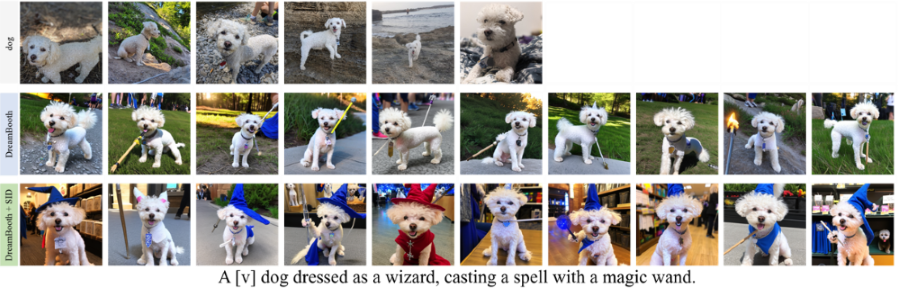}
    \vspace{0.2cm}

    \caption{diverse but entangled, 1st (backgound mountain), 2nd (rocky surface), 3rd (nearby teapot, saurcer, filled in flower), last ( grassy field)}
    % \label{fig:vs_Neg_Seg}
\end{figure*}
