# Supplementary material for: Selectively Informative Description can Reduce Undesired Embedding Entanglements in Text-to-Image Personalization
Source: arXiv:2403.15330 source file (2024-03-22)
Supplement: Supplementary file 3 [file 938_1.Multi_vs_DB_diverse_not.tex]

\begin{figure*}[t]
    \centering
    \includegraphics[width=0.9\textwidth]{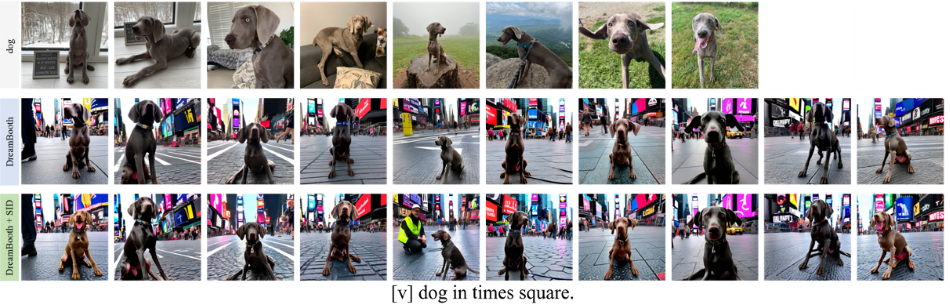}
    \vspace{0.2cm}

    \includegraphics[width=0.9\textwidth]{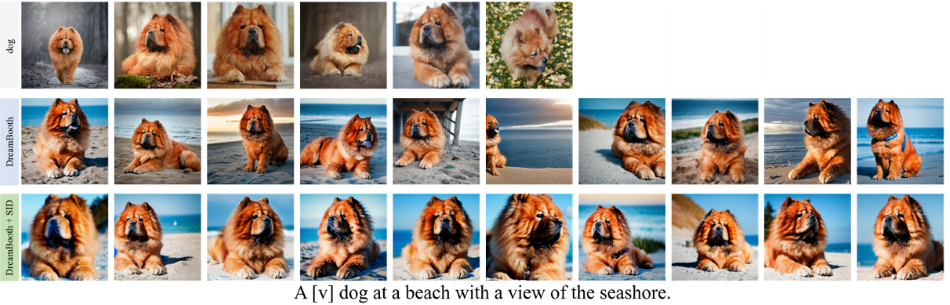}
    \vspace{0.2cm}

    \includegraphics[width=0.9\textwidth]{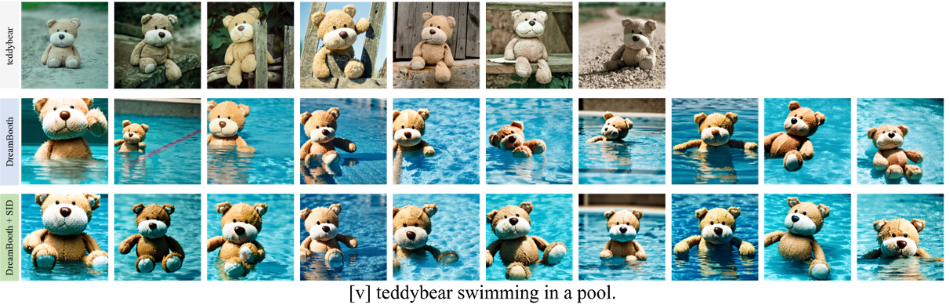}
    \vspace{0.2cm}

    \includegraphics[width=0.9\textwidth]{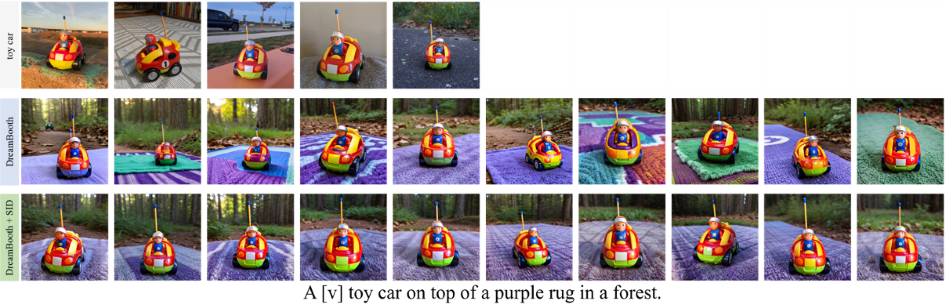}
    \vspace{0.2cm}

    \caption{biased examples}
    % \label{fig:vs_Neg_Seg}
\end{figure*}
