# Supplementary material for: Selectively Informative Description can Reduce Undesired Embedding Entanglements in Text-to-Image Personalization
Source: arXiv:2403.15330 source file (2024-03-22)
Supplement: Supplementary file 4 [file X0.Quantitative_analysis_Fig2.tex]

\section{Quantitative comparison between the description cases.}
To perform quantitative comparison on ~~~.
9개의 subject, 각 subject 당 4~6장 이미지, subject에 속하는 이미지가 거의 비슷한 content를 공유하는 bias가 심한 이미지로 선별
이렇게한 이유는 bias가 심한 challenging한 상황을 고려하기 위해, 여러 이미지에 대해 하나의 training description만 사용해서 분석의 편의성을 높이기 위해.
% \input{Suppl_TEX/01.Table_Quantitative_Fig2}

% use 9 subject, each subject consist of 4~6 reference images, and 
