# Supplementary material for: Selectively Informative Description can Reduce Undesired Embedding Entanglements in Text-to-Image Personalization
Source: arXiv:2403.15330 source file (2024-03-22)
Supplement: Supplementary file 5 [file X0.Random_Multi.tex]

...

\begin{figure*}[t]
\centering
\includegraphics[width=0.9\textwidth]{Figures/overall.png}
\vspace{0.2cm}

\includegraphics[width=0.9\textwidth]{Figures/overall.png}
\vspace{0.2cm}

\includegraphics[width=0.9\textwidth]{Figures/overall.png}
\vspace{0.2cm}

\includegraphics[width=0.9\textwidth]{Figures/overall.png}
\caption{hello}
\label{fig:prompt_ablation_blueberry_bowl}
\end{figure*}
